# Supplementary material for: Three-dimensional dopant distribution from a single, out-of-focus spectroscopic image
Source: arXiv:2610.11053 source file (2026-10-08)
Supplement: Supplementary file 1 [file Experimental_Details.tex]

\section{Experimental Details}\label{sec:exp-details}

\subsection{Sample Preparation}

The sample was a Fe-doped MgAl$_2$O$_4$ crystal, synthesized at the Commonwealth Scientific and Industrial Research Organisation and supplied by Peter Miller. The crystal was crushed to create small shards. To avoid silicate contamination, a sufficiently hard zirconia mortar and pestle was used for crushing, with the sample dispersed in pure ethanol. Settling time was deliberately shortened to drop cast larger shards, exceeding several microns, onto a holey cardon film supported on a 400 mesh 3.05mm copper grid, to enable easier tilting onto crystal zone axes. To diminish experimental artefacts, several additional preparation steps were undertaken before and after drop casting. Firstly, the holey carbon film was pre-cleaned using pure ethyl acetate to remove hydrocarbons potentially arising from residual polyvinyl formal (Formvar). To improve thermal and electrical conductivity, an AuPd sputter target was employed to half-coat the holey carbon support by Julian Ratcliffe, prior to drop casting, giving rise to a continuous gradation in the concentration of AuPd nanocrystals across the grid ranging from nascent to a continuous AuPd film. Lastly, to ameliorate previously observed specimen instability, plasma cleaning of the drop-cast specimen was avoided and, instead, the sample was heated to 120°C ex-situ, effecting an ultrathin conductive coating of carbon and removal of moisture.


\subsection{Microscope and Acquisition Details}

The sample was characterised using a Thermo Scientific Spectra $\varphi$ monochromated, dual aberration corrected field emission gun transmission electron microscope. The EELS spectra were acquired using a Gatan Continuum K3 HR spectrometer, fitted with a K3 direct electron detection camera. A spectrometer collection semi-angle of 69mrad was used. Spectra were acquired in single EELS mode to reduce dose overhead. A dispersion of 0.9eV per pixel was used to maximise signal per bin, with an energy loss range from ~370eV to ~3100eV. This collects the Fe L$_{2,3}$ edge shown here, but also the O-K, Mg-K and Al-K edges. An exposure time of 20ms per spectra was used. Suitable areas for study were screened for thickness by collection of $t/\lambda$ maps. Precise, to within a unit cell, thickness measurement was carried out by matching energy filtered position averaged convergent beam electron diffraction (PACBED) patterns (shown in \cref{sec:fig:fov_exam} of \cref{sec:examining-fov}), acquired using a Gatan K3 direction electron detection camera, to simulated patterns. 
